# Supplementary material for: Color-Perception-Guided Display Power Reduction for Virtual Reality
Source: arXiv:2209.07610 source file (2022-09-19)
Supplement: Supplementary file 1 [file sec_supp.tex]

\onecolumn
\section{Optimal Color Modulation Derivation}
\label{appn:optimal-derivation}

Given an ellipse constraint function
%
\begin{align}
\begin{cases}
\ellipse(\colorVec)
= \left(\frac{\colorCoordinate_1 - \testCoordinate_1}{\ellipseCoordinate_1}\right)^2
+ \left(\frac{\colorCoordinate_2 - \testCoordinate_2}{\ellipseCoordinate_2}\right)^2
- 1 = 0\\
\colorCoordinate_3 = \testCoordinate_3,
\end{cases}
\end{align}
%
and a power cost function
%
\begin{align}
\power(\colorVec)
= \powerCoordinate_1 \colorCoordinate_1 + \powerCoordinate_2 \colorCoordinate_2 + \powerCoordinate_3 \colorCoordinate_3 + \powerCirc,
\end{align}
%
we may solve the power optimizing $\colorVec^*$ via the method of Lagrange multipliers.

First, we notice that $\colorCoordinate_3$ should not change.
Intuitively, this effectively reduces the dimensionality of the optimization onto the plane $\colorCoordinate_3 = \testCoordinate_3$.
Formally, we may rewrite the constraint and power functions in terms of a 2-dimensional variable $\vec{y} = (y_1, y_2) = (\colorCoordinate_1, \colorCoordinate_2)$:
%
\begin{align}
\ellipse(\vec{y})
= \left(\frac{y_1 - \testCoordinate_1}{\ellipseCoordinate_1}\right)^2
+ \left(\frac{y_2 - \testCoordinate_2}{\ellipseCoordinate_2}\right)^2
- 1 = 0,
\end{align}
%
and
%
\begin{align}
\power(\vec{y}) = \powerCoordinate_1 y_1 + \powerCoordinate_2 y_2 + const.
\end{align}

The minimizing vector $\vec{y}^*$ satisfies the condition that the gradients of $\ellipse$, and $\power$ are co-linear.
So the system of equations we need to solve for $\vec{y}^*$ is
%
\begin{align}
\begin{cases}
\nabla \ellipse(\vec{y}^*) = \phi \nabla \power(\vec{y}^*)\\
\ellipse(\vec{y}^*) = 0,
\end{cases}
\end{align}
%
for some scalar constant $\phi$.

Computing the gradients, we get
%
\begin{align}
\begin{cases}
\frac{2}{\ellipseCoordinate_1} \frac{y_1^* - \testCoordinate_1}{\ellipseCoordinate_1} = \phi \powerCoordinate_1\\
\frac{2}{\ellipseCoordinate_2} \frac{y_2^* - \testCoordinate_2}{\ellipseCoordinate_2} = \phi \powerCoordinate_2\\
\left(\frac{y_1^* - \testCoordinate_1}{\ellipseCoordinate_1}\right)^2
+ \left(\frac{y_2^* - \testCoordinate_2}{\ellipseCoordinate_2}\right)^2
- 1 = 0.
\end{cases}
\end{align}

Finally, we solve for $\vec{y}^*$ using this system of equations to get the optimal color, $\vec{x}^*$:
%
\begin{align}
\begin{aligned}
x_1^* &= \frac{\powerCoordinate_1 \ellipseCoordinate_1^2}{\sqrt{\powerCoordinate_1^2\ellipseCoordinate_1^2 + \powerCoordinate_2^2\ellipseCoordinate_2^2}}\\
x_2^* &= \frac{\powerCoordinate_2 \ellipseCoordinate_2^2}{\sqrt{\powerCoordinate_1^2\ellipseCoordinate_1^2 + \powerCoordinate_2^2\ellipseCoordinate_2^2}}\\
x_3^* &= \testCoordinate_3.
\end{aligned}
\end{align}

\section{Individual participant data for pilot perceptual user study}
\label{sec:supp:pilot-individual}

\begin{longtable}{ c c c c }
    Subject ID & \hspace{1em}Eccentricity $= 10^\circ$ & \hspace{1.5em}Eccentricity $= 25^\circ$ & \hspace{1.3em}Eccentricity $= 35^\circ$\\
    
    \hline
    \\
    subject\_01 &
    \begin{minipage}{0.26 \textwidth}
        \includegraphics[width=\linewidth]{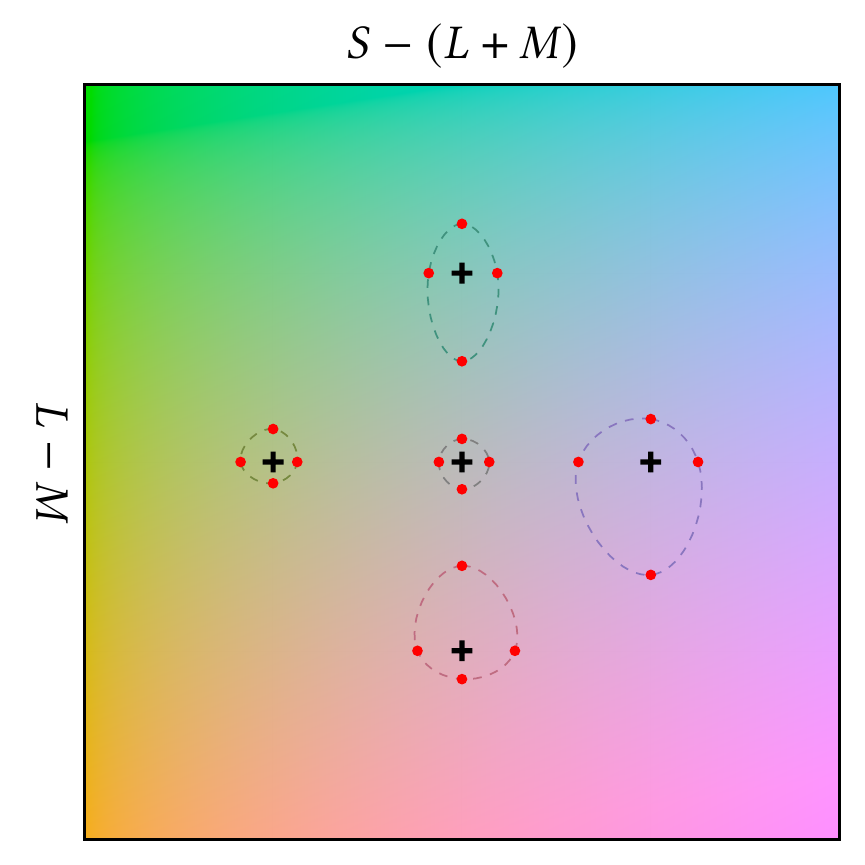}
    \end{minipage}
    &
    \begin{minipage}{0.26 \textwidth}
        \includegraphics[width=\linewidth]{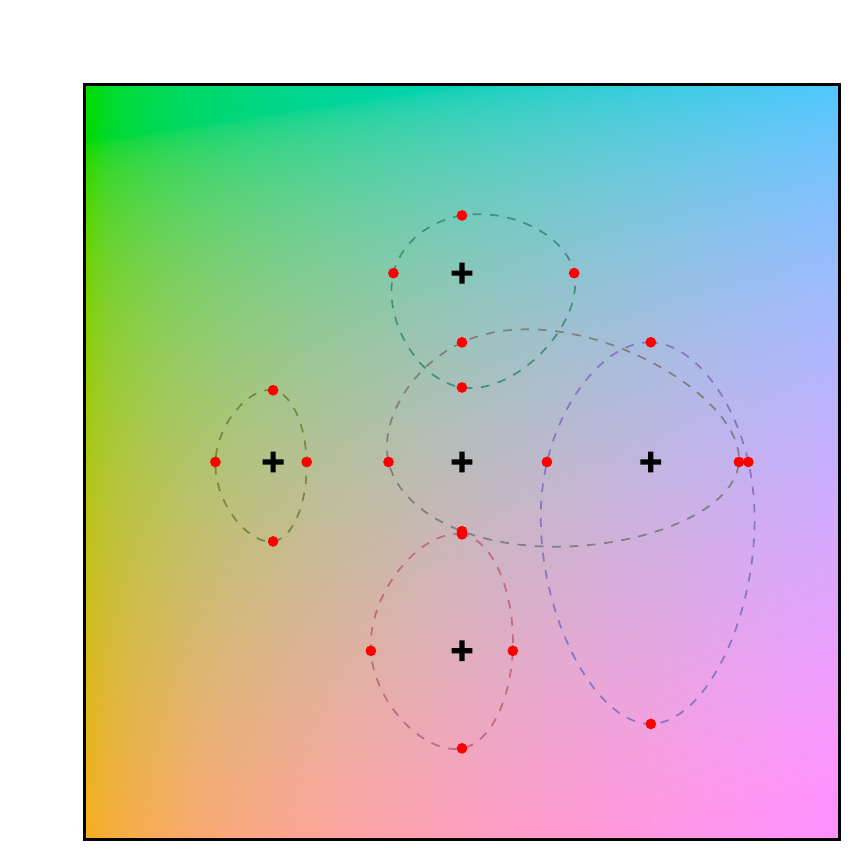}
    \end{minipage}
    &
    \begin{minipage}{0.26 \textwidth}
        \includegraphics[width=\linewidth]{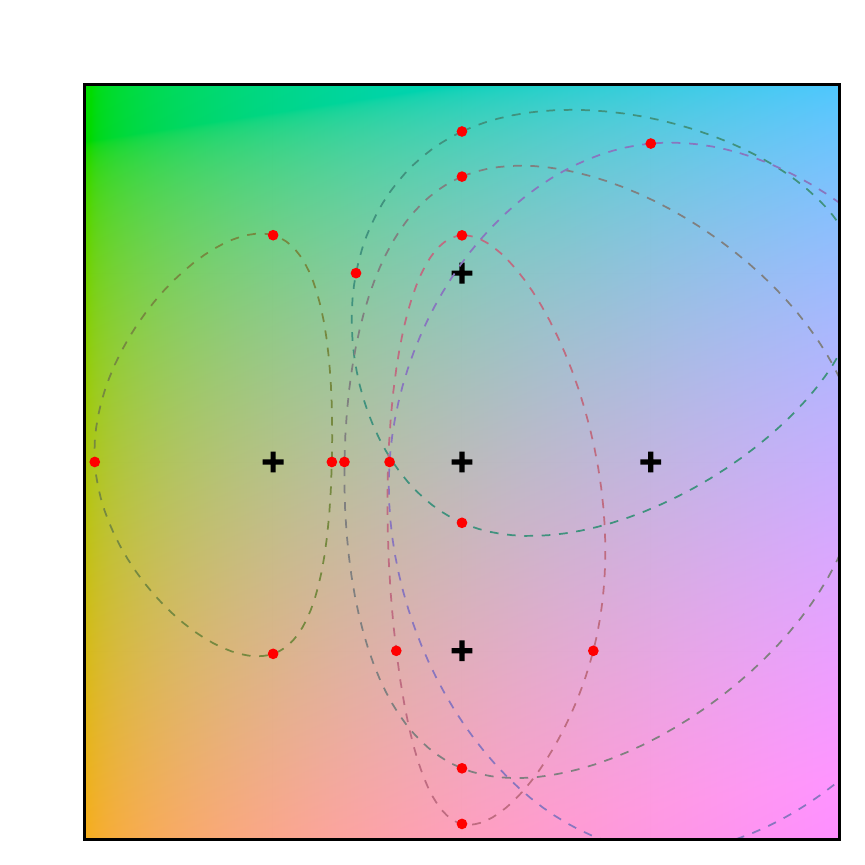}
    \end{minipage}
    \\
    
    subject\_02 &
    \begin{minipage}{0.26 \textwidth}
        \includegraphics[width=\linewidth]{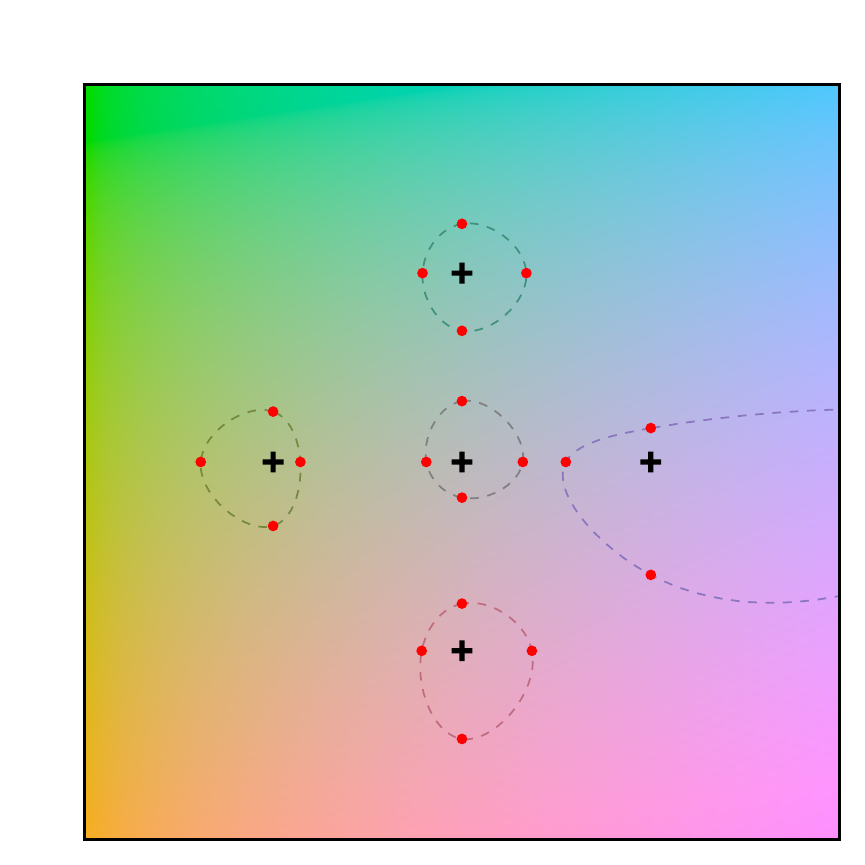}
    \end{minipage}
    &
    \begin{minipage}{0.26 \textwidth}
        \includegraphics[width=\linewidth]{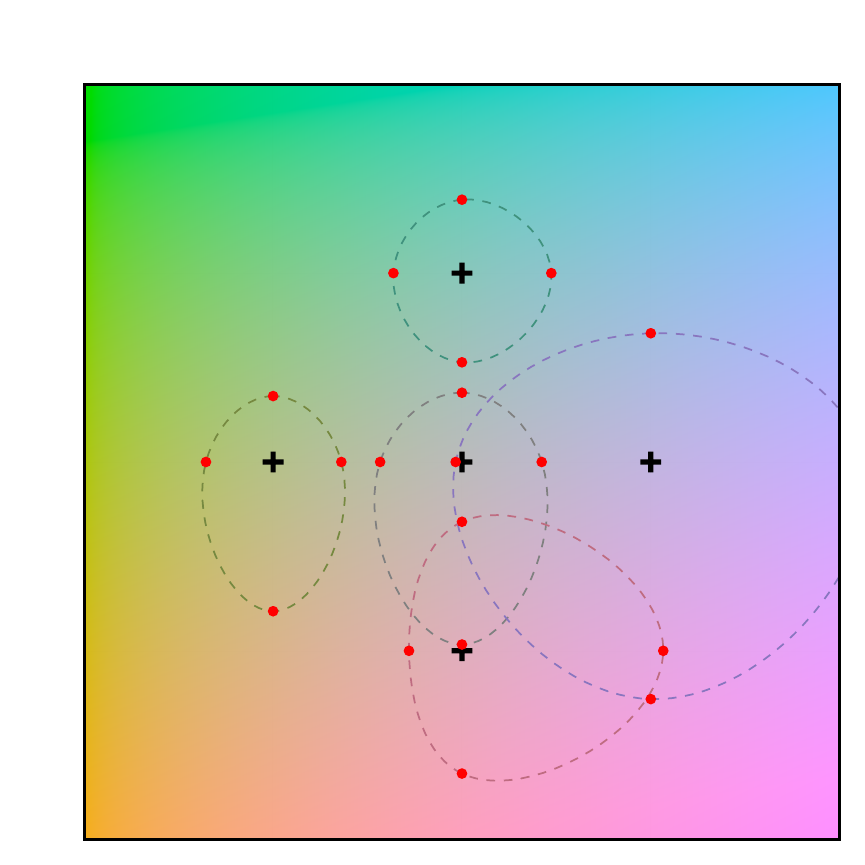}
    \end{minipage}
    &
    \begin{minipage}{0.26 \textwidth}
        \includegraphics[width=\linewidth]{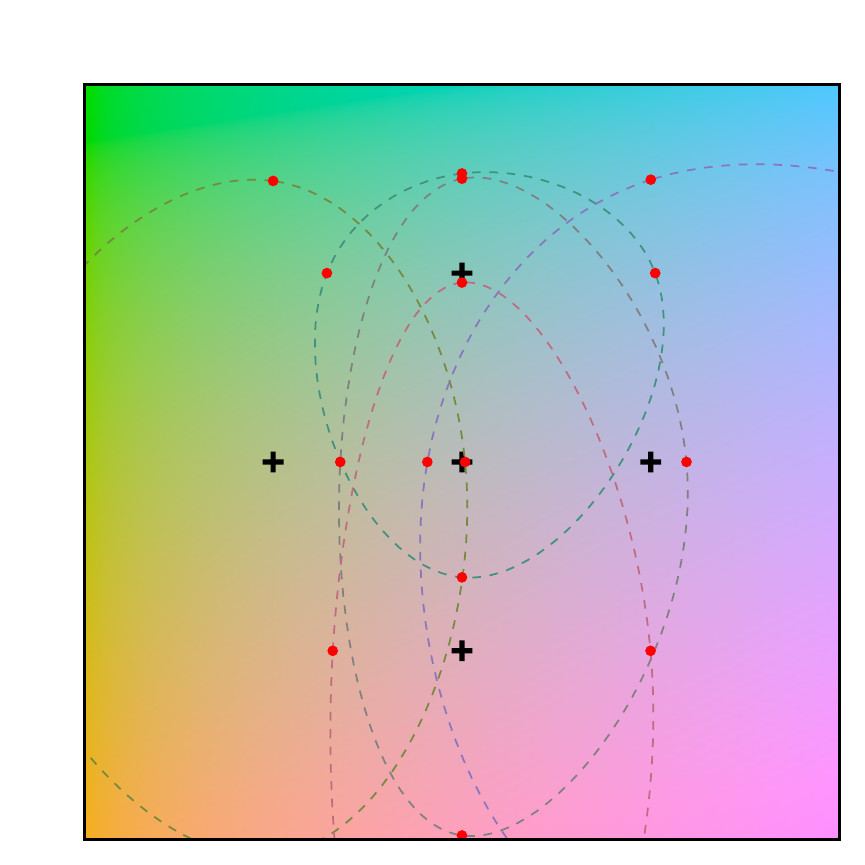}
    \end{minipage}
    \\
    
    subject\_03 &
    \begin{minipage}{0.26 \textwidth}
        \includegraphics[width=\linewidth]{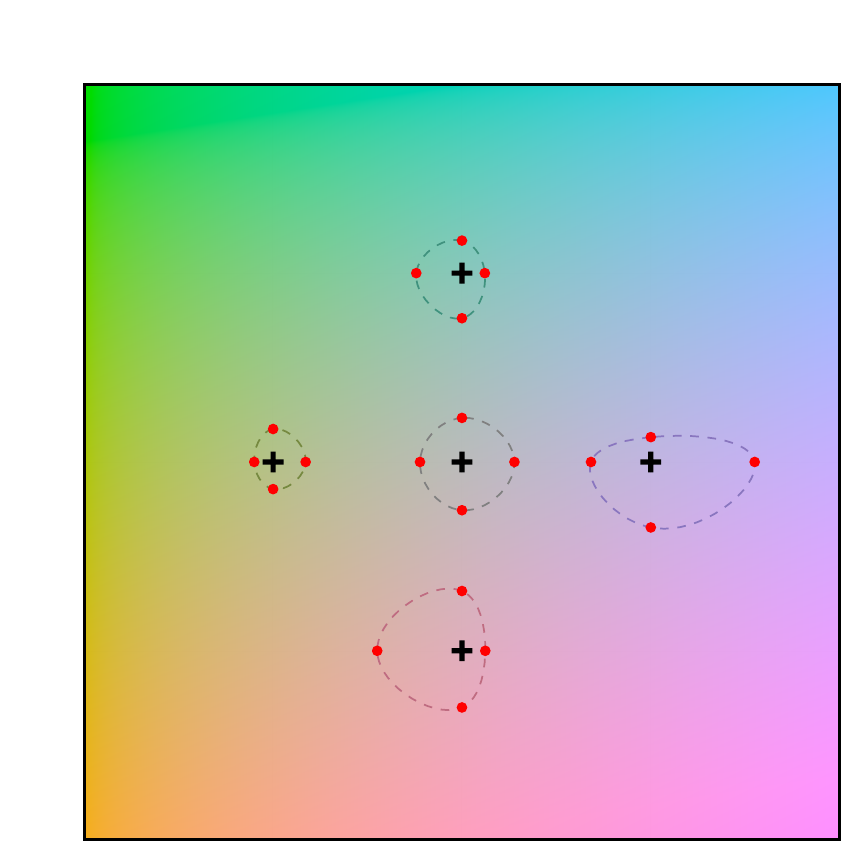}
    \end{minipage}
    &
    \begin{minipage}{0.26 \textwidth}
        \includegraphics[width=\linewidth]{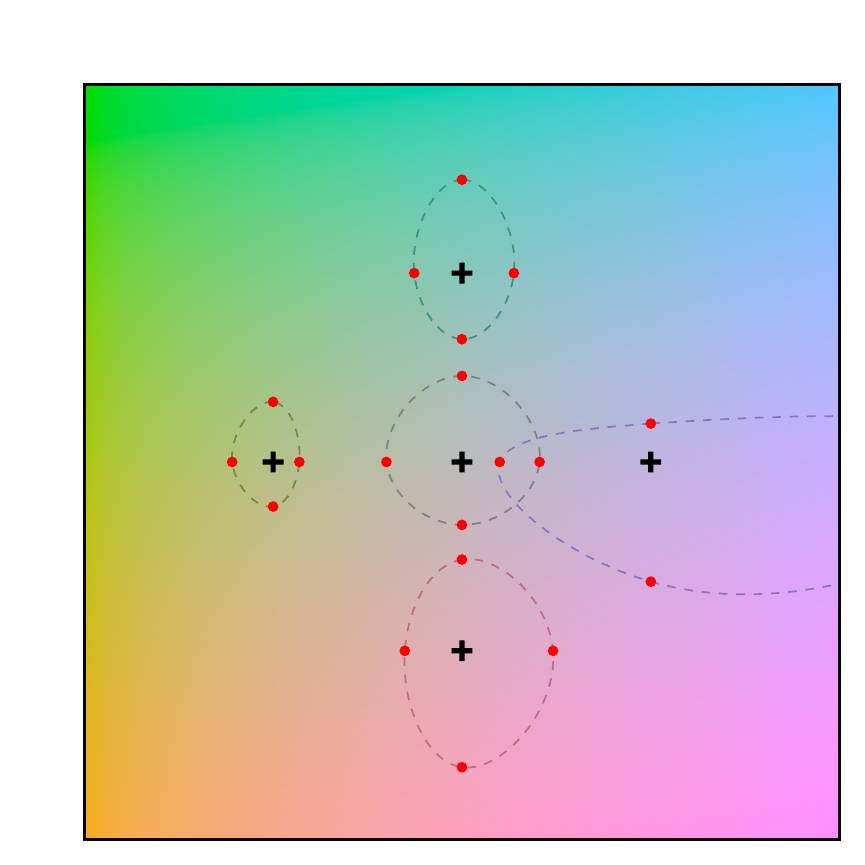}
    \end{minipage}
    &
    \begin{minipage}{0.26 \textwidth}
        \includegraphics[width=\linewidth]{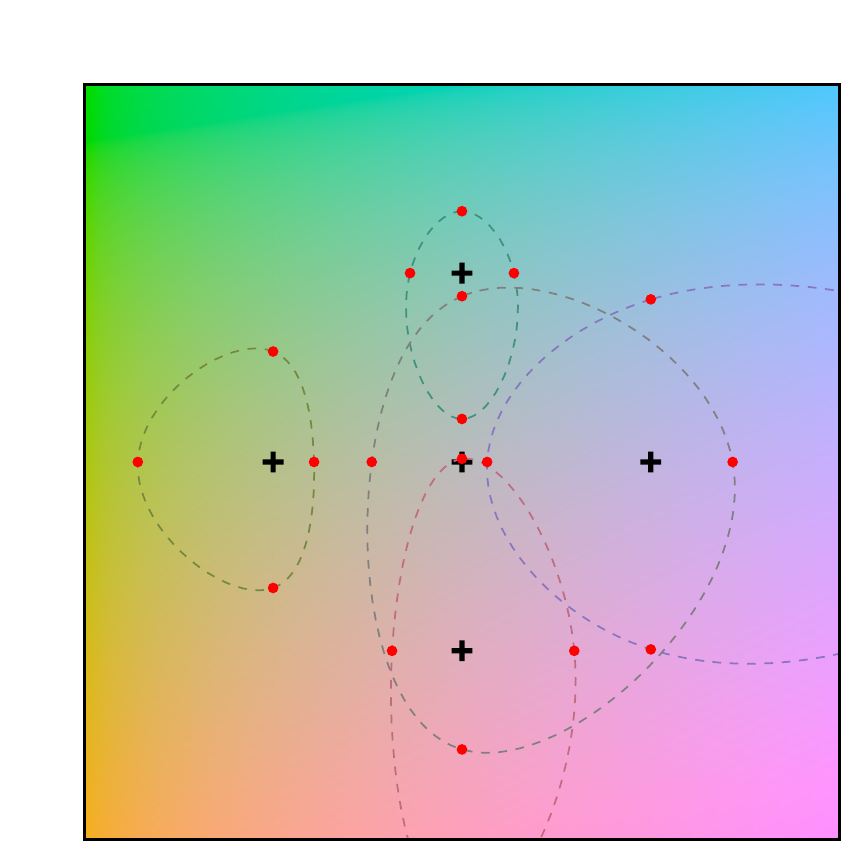}
    \end{minipage}
    \\
    
    subject\_04 &
    \begin{minipage}{0.26 \textwidth}
        \includegraphics[width=\linewidth]{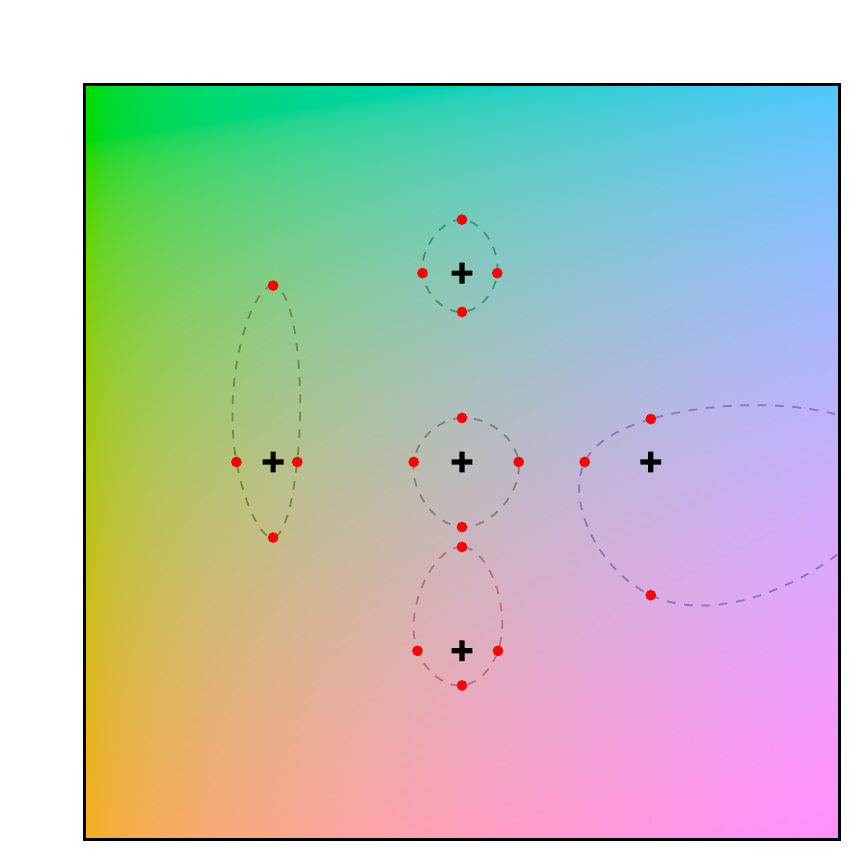}
    \end{minipage}
    &
    \begin{minipage}{0.26 \textwidth}
        \includegraphics[width=\linewidth]{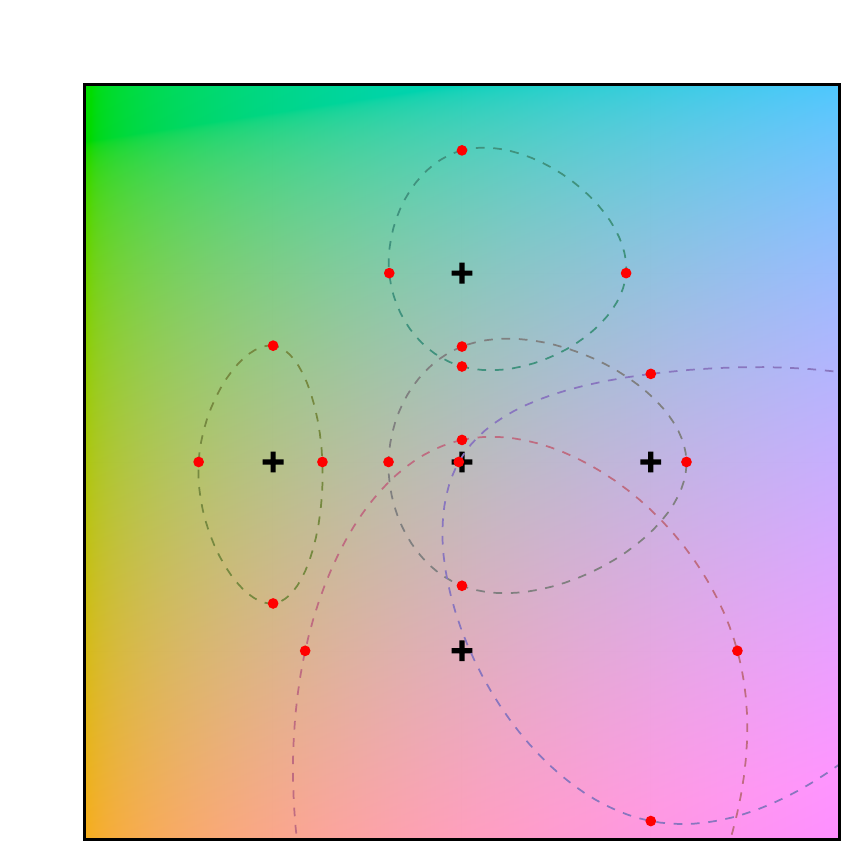}
    \end{minipage}
    &
    \begin{minipage}{0.26 \textwidth}
        \includegraphics[width=\linewidth]{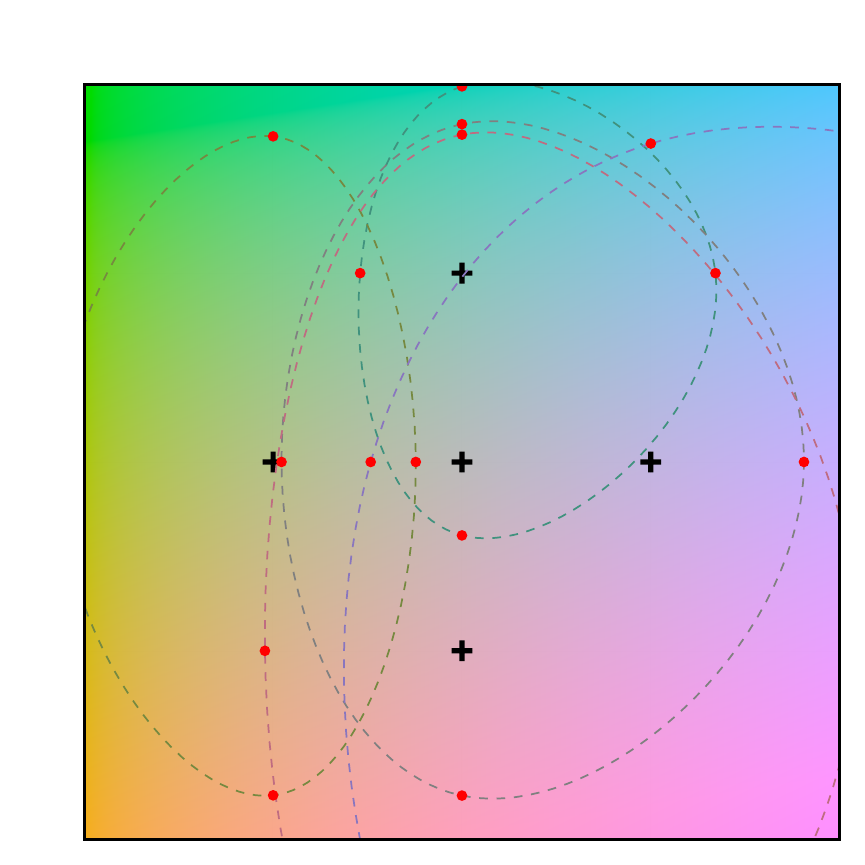}
    \end{minipage}
    \\
    
    subject\_05 &
    \begin{minipage}{0.26 \textwidth}
        \includegraphics[width=\linewidth]{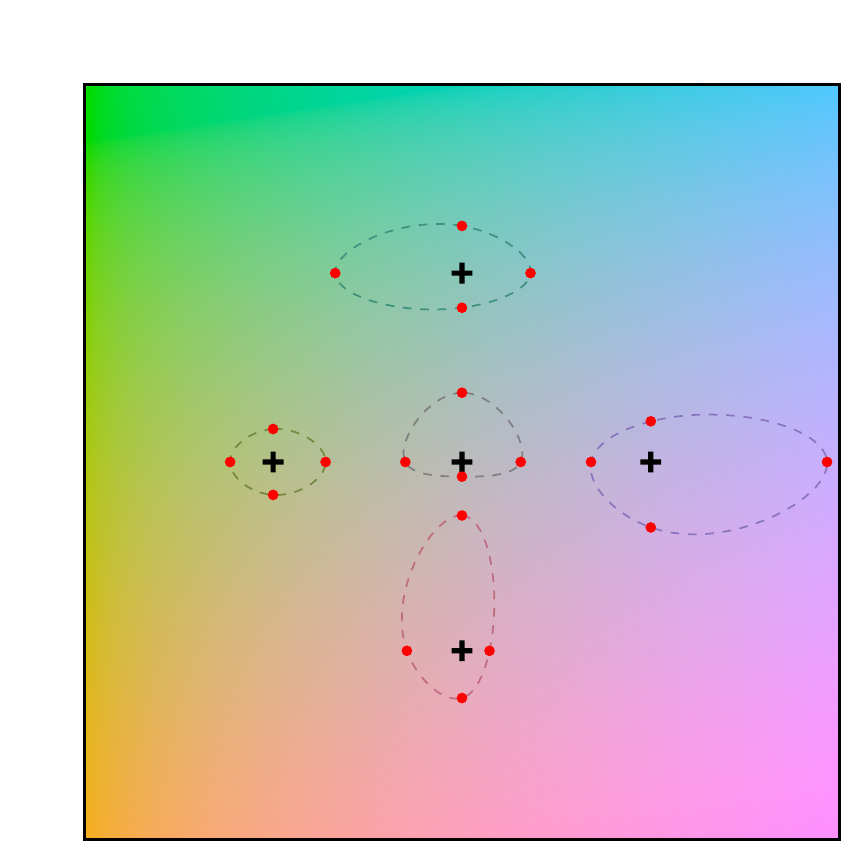}
    \end{minipage}
    &
    \begin{minipage}{0.26 \textwidth}
        \includegraphics[width=\linewidth]{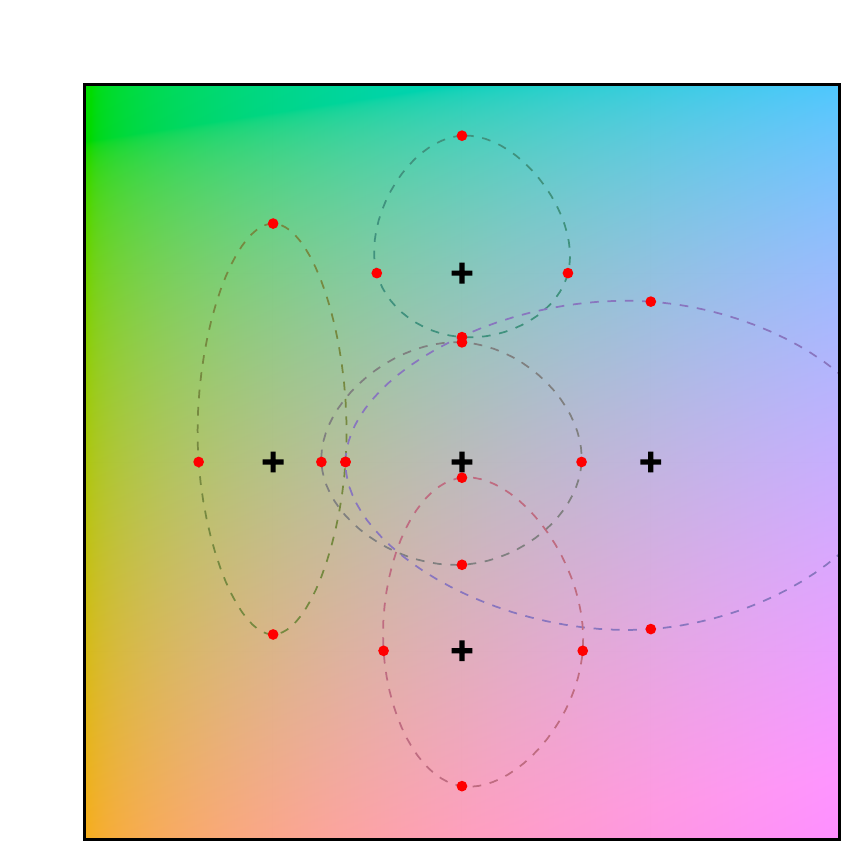}
    \end{minipage}
    &
    \begin{minipage}{0.26 \textwidth}
        \includegraphics[width=\linewidth]{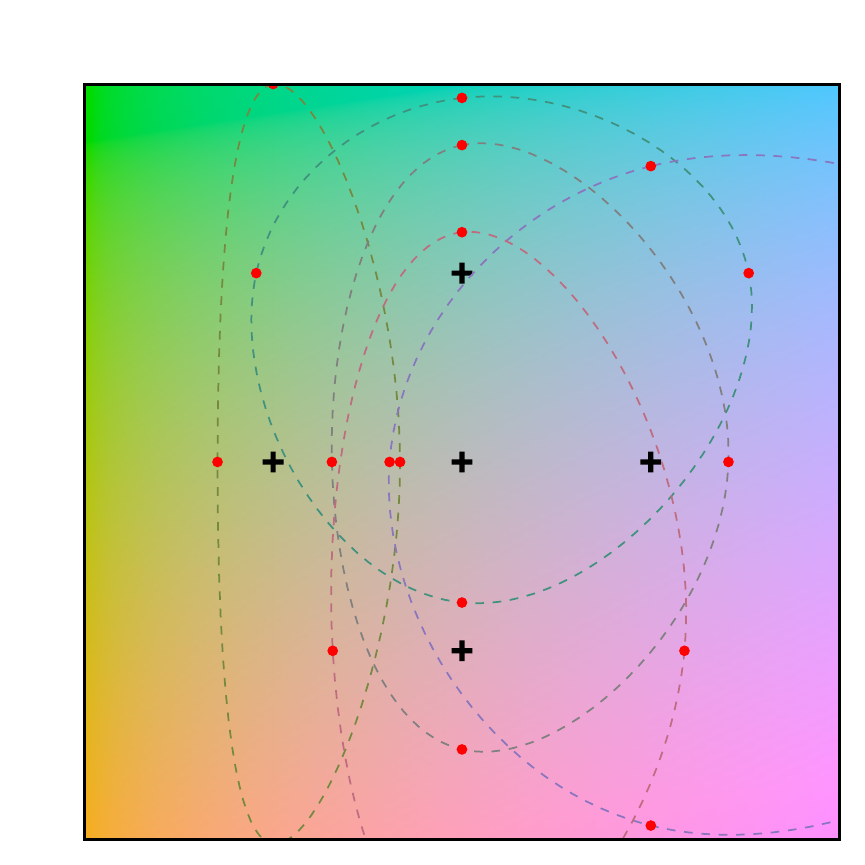}
    \end{minipage}
    \\
\caption{\label{fig:supp:pilot_data} Pilot Perceptual Study Threshold Data}
\end{longtable}
